# Supplementary material for: MemorySeg: Online LiDAR Semantic Segmentation with a Latent Memory
Source: arXiv:2311.01556 source file (2023-11-02)
Supplement: Supplementary file 1 [file supp_ablations.tex]

\section{Addtional Ablations}
